# Supplementary material for: Enabling Cooperative Hybrid Beamforming in TDD-based Distributed MIMO Systems
Source: arXiv:2308.15659 source file (2023-08-29)
Supplement: Supplementary file 1 [file appendix.tex]

\section*{Appendix I}
\label{sec:appendix}

We will start by a few supplementary definitions that are required for the proof of Theorem~\ref{lemma:Tulip_2}.
% \begin{defn}
% A contiguous beam, say scanning beam, is denoted by its angular coverage interval (ACI). For example a beam $i$ is denoted as $[s_i,e_i)$ where $s_i$ is the starting point (angle) and $e_i$ is the ending point (angle). 
% \label{defn: contiguous}
% \end{defn}

\begin{defn}
A direction is defined on the azimuth angles, say, counter-clockwise. The ACI as well as the starting and the ending point of a beam is measured with respect to this direction. For example, one may have a beam starting at $3\pi/2$ and ending at $\pi/2$ which is represented as $[ 3 \pi /2, \pi/2)$.
\label{defn: loop}
\end{defn}

\begin{defn}
Consider a set of points $a_1, a_2, \ldots, a_n$, $n\geq3$ on a circle. For any three indices $1 \leq i, j, k \leq n$, we write $a_i \prec a_j \prec a_k$ (and read as  $a_i$ precedes $a_j$ precedes $a_k$) if by starting from point $a_i$ and moving in the defined direction (say counter clockwise) we first encounter $a_j$ and then encounter $a_k$ before reaching $a_i$ again. Equivalently, we write $a_k \succ a_j \succ a_i$ and read $a_k$ succeeds $a_j$ succeeds $a_i$. Please note that the precedence relation requires at least three points to be specified.
\label{defn: prec_succ}
\end{defn}

\begin{defn}
Consider $b$ beams and denote them by beam $i$, $i \in B$ where $B = {1, 2, \ldots, b}$ denotes the set of all possible beam. For a given subset $C \subset B$, we define a component beam $\omega_C$ as a beam (possibly comprised of an interval or a collection of intervals) where each differential arc of the beam contains all the beams in $C$ and does not contain any beam which is not in $C$. The set $C$ is called the \emph{spawning set} of $\omega_C$ and its cardinality is called the \emph{degree} of $\omega_C$. A component beam with spawning set $C$ may or may not exist, and if it exist we may refer to the component beam by its spawning set $C$.  We say a \emph{component beam has a beam $i$ in its intersection} if the beam $i$ belongs to its spawning set.
\label{defn:component}
\end{defn}

\begin{defn}
We define the following operators and notations on spawning set. Let a spawning set (or equivalently a component beam) be denoted by capital letters $C, D, E, F, X, Y$, etc., and a set of spawning sets be represented by $\mathcal{C}, \mathcal{E}$, etc., e.g., $\mathcal{C} = \{C, D\}$, and $\mathcal{E} = \{E, F\}$. The union of two spawning set $C \cup D$ is denoted by $CD$. The cross product (or product or union product) of two sets of spawning sets $\mathcal{C}$ and $\mathcal{E}$ is denoted by $\mathcal{C} \times \mathcal{E}$ and is defined as a set that contains the union of any pair of sets such that one set belongs to the first and the other one belongs to the second set of spawning sets, i.e., $\mathcal{C} \times \mathcal{E} = \{X, X = X_1 X_2, X_1 \in \mathcal{C}, X_2 \in \mathcal{D}\}$. For example $\{C,D\} \times \{E,F\} = \{CE, CF, DE, DF\}$. The multiplication of the set of spawning sets $\mathcal{C}$ by itself may be represented as $\mathcal{C}^2 = \mathcal{C} \times \mathcal{C}$. The higher power $k > 2$ may be defined recursively as $\mathcal{C}^k = \mathcal{C}^{k-1} \times \mathcal{C}$.
\label{defn:product}
\end{defn}

If a set of spawning sets $\mathcal{D}$ contains a single spawning set $C$ it may be represented by $C$ instead of $\mathcal{D}$. Similarly, if a spawning set contains a single beam $c$, i.e., $C = \{ c\}$ it may be directly represented by $c$ instead of $C$. The definition of the operators $\setminus$ and $\times$ is inherited for the spawning sets and beams as well. For example, we may write $C \times \mathcal{D}$ where in this expression $C$ is interpreted as a set of spawning set which contains a single spawning set $C$. We denote the set minus operation by $-$, i.e., $C - D = \{x, x \in C, x \notin D \}$. We assume that the operator $\setminus$ has precedence on the operators $\times$, $\cup$, $\cap$, and $-$ , e.g., $C \times \mathcal{D} E = C \times (\mathcal{D} \setminus E)$

\begin{lemma}
Among the set of contiguous scanning beams, a set of scanning beams with Tulip design generates the maximal number of possible feedback sequences for the channel with $p = 1$ path.
\label{lemma:Tulip_1}
\end{lemma}

\proof
The proof relies on the fact that $b$ contiguous beams have total of $2b$ starting and ending points and hence can generate at most $2b$ component beams. On the other hand for $p=1$ a feedback sequence is valid only and only if the set of the indices of the beam with positive feedback corresponds to an spawning set of a component beam that is realized by the set of scanning beams. Since there are at most $2b$ component beam, there is only $2b$ possible feedback sequences and Tulip design already provides $2b$ component beams. We note that the Tulip structure is not the only optimal design for $p=1$.

\begin{lemma}
For a channel with $p=2$ paths, a set of scanning beams with Tulip design generates $1, 3, 7$, and  $15$ feedback sequences for $b = 1, 2, 3$, and 4 beams, respectively, and generates $2b(b-2)$ feedback sequences for $b > 4$ beams. 
\label{lemma:Tulip_2_count}
\end{lemma}

\proof
The proof is simply follows from a direct counting argument.
There are $b$ component beams of degree 1 with spawning sets $\{1\}, \{2\}, \ldots, \{b\}$ that are directly part of the Tulip design. For $b>1$, there are $b \choose 2$ feedback sequences of degree 2 corresponding to the beam index sets $\{12\}, \{13\}, \ldots, \{1b\}, \{23\}, \{24\}, \ldots, \{2b\}, \ldots, \{(b-1)b\}$. A degree 2 feedback sequence corresponding to an index set $\{ij\}$ can be generated by selecting path 1 and path 2 inside the component beams $\{i\}$ and $\{j\}$, respectively. For $b > 2$, a feedback sequence of degree 3 may be generated by selecting a path in a component beam of degree 2 and a path in a component beam of degree $1$. In the following consider the indices of the beam in mod $b$. In other words, the beam $b+1$ is the same as beam $1$. There are total of $b(b-3)$ feedback sequences of type $i(i+1)k$. Consider the set $C_i = \{ i(i+1)k, k \neq i, k \neq (i+1)\}$. There are $b$ sets $C_i, i = 1, 2, \ldots, b$, and each set $C_i$ has $b-2$ distinct feedback sequences and there are exactly $b$ feedback sequences of the form $i(i+1)(i+2)$ which appear in all sets 
$C_i, i = 1, 2, \ldots, b$ exactly twice. Hence the union $\cup_{i \on B} C_i$ contains exactly $b(b-3)$ distinct feedback sequences. Similarly, for $b>4$, it can be argued that there are exactly $b(b-3)/2$ degree 4 feedback sequences of type $i(i+1)j(j+1)$, $i+1 \succ j$, $j+1 \succ i$ that are generated by having one path in the component beam $i(i+1)$ and another in the component beam $j(j+1)$. For $b=4$, there is only one feedback sequence $1234$ that is generated by having one path in component beam $12$ and one path in component beam $34$. Summing all the feedback sequences of degree 1 to degree 4 proves the statement of the lemma.

% \begin{lemma}[NOT REQUIRED]
% For a set of scanning beam $\{[s_1,e_1),[s_2,e_2),\ldots,[s_b,e_b),\}$ where $s_1 \prec s_2 \prec \ldots \prec s_b$, if the beam $j$ is the first nested beam in beam $i$, then exchanging the beam $i$ and $j$ with the two new beams $[s_i,e_j)$ and $[s_j, e_i)$, the number of possible feedback sequences is not decreased. 
% \label{lemma: nested}
% \end{lemma}

% \proof

\subsection*{\textbf{Proof of Theorem~\ref{lemma:Tulip_2}:}}
Lemma~\ref{lemma:Tulip_1} proves the optimality of Tulip design for a channel with single path, i.e., $p=1$. Lemma~\ref{lemma:Tulip_2}, extends this optimality to the case of $p=2$, however, the proof is considerably more involved. 

Here, we first provide the sketch of the proof and then formally get into the details. Lemma~\ref{lemma:Tulip_2_count}, counts the number of feedback sequences that is generated by Tulip design. It is relatively easy to check for small numbers of $b \leq 5$ that no other set of scanning beams can generate more number of feedback sequences as Tulip design. For the case of $b>5$, we prove the theorem by using the following steps.

Consider a set of $b$ contiguous scanning beams $\mathcal{B}$ positioned on a circle. Let $\mathcal{C}$ denote the set of component beams generated by the set of scanning beams $\mathcal{B}$. 

First, we note that without loss of generality we can assume that set of starting and ending point of each scanning beam interval, i.e., \emph{end point markers}, are disjoint, which means that every starting point and ending point is unique. Suppose not; consider the ordered set of end point markers $x_1 \succ x_2 \succ \ldots \succ x_{2b}$ and assume that two consecutive points $x_i$ and $x_j$ (say $x_1$ and $x_2$ or $x_{2b}$ and $x_1$) are equal $x_i = x_j$ and we have $x_{i-1} \succ x_i \succ x_{j+1}$. Consider two cases: (i) At least one of the points $x_i$ and $x_j$ are an ending point. Let $x_j$ be an ending point. By moving it to point $x_j'$ such that $x_i \succ x_j' \succ x_{j+1}$, one can generate an extra component beams. (ii) Both $x_i$ and $x_j$ are an starting point. By moving $x_i$ to point $x_i'$ such that $x_{i-1} \succ x_i' \succ x_j$, one can generate an extra component beams. In either case (i) or case (ii), by adding a new component beam to the set $\mathcal{C}$, the cardinality of $\mathcal{C}^2$ cannot decrease. 

Hence, we can assume that in the maximal case of $\mathcal{C}$, its cardinality is exactly $2b$. In other words, there exist a $\mathcal{C}$ which is maximal, i.e., $|\mathcal{C}^2|$ is maximum when $|\mathcal{C}| = 2b$. It can be easily verified that when considering $2b$ the component beams on the loop, the spawning sets of any two consecutive component beam $C_i$ and $C_{i+1}$ differ only in one element which means that (i) either $C_i \subset C_{i+1}$ or $C_i \supset C_{i+1}$ and (ii) $||C_i| - |C_{i+1}|| = 1$.

\emph{Claim 1}: Consider a subset $\mathcal{A} = \{A_1, \ldots, A_n\}$ of $n$ elements of the $\mathcal{C}$ that are adjacent in the loop. If we add a new spawning set $A$ to one end of the loop (without loss of generality assume to the right hand side of the loop), and $|A| < |A_n|$, then $|(\mathcal{A} \cup A)^2| \leq |\mathcal{A}^2| + n-2$. One of the following four cases might have occurred, and in each case all three unions $A \cup A_n$, $A \cup A_{n-1}$, and $A \cup A_{n-2}$ are repeated in some other combinations and hence they do not generate a new spawning set in $(\mathcal{A} \cup A)^2$. We have (i) $A_{n-2} \supset A_{n-1} \supset A_{n} \supset A$ in which case $A \cup A_n = A_n$, $A \cup A_{n-1} = A_{n-1}$, and $A \cup A_{n-2} = A_{n-2}$; (ii) $A_{n-2} \subset A_{n-1} \supset A_{n} \supset A$ in which case $A \cup A_n = A_n$, $A \cup A_{n-1} = A_{n-1}$, and $A \cup A_{n-2} = A_{n-2}$ or $A_{n-1}$; (iii) $A_{n-2} \subset A_{n-1} \subset A_{n} \supset A$ in which case $A \cup A_n = A_n$, $A \cup A_{n-1} = A_{n}$, and $A \cup A_{n-2} = A$ or $A_{n-2}$; (iv) $A_{n-2} \supset A_{n-1} \subset A_{n} \supset A$ in which case $A \cup A_n = A_n$, $A \cup A_{n-1} = A_{n}$, and $A \cup A_{n-2} = A_n \cup A_{n-2}$. Hence, at most $n-3$ new subsets of the form $A_i \cup A, 1 \leq i \leq n-3$ and one new subset corresponding to the new subset $A$ are generated.

\emph{Claim 2}: Consider a subset $\mathcal{A} = \{A_1, \ldots, A_n\}$ of $n$ elements of the $\mathcal{C}$ that are adjacent in the loop. If we add a new spawning set $A$ to one end of the loop (without loss of generality assume to the right hand side of the loop), and $|A| > |A_n|$, then $|(\mathcal{A} \cup A)^2| \leq |\mathcal{A}^2| + n-1$ or $|(\mathcal{A} \cup A)^2| \leq 2n$ . One of the following three cases might have occurred. We have (i) $A_{n-1} \subset A_{n} \subset A$ in which case $A \cup A_n = A$, $A \cup A_{n-1} = A$; (ii) $A_{n-2} \subset A_{n-1} \supset A_{n} \subset A$ in which case $A \cup A_n = A$ and $A \cup A_{n-2} = A \cup A_{n-1}$; (iii) $\exist i, i \geq 1$ such that $A_i \subset A_{i+1} \supset \ldots \supset A_{n-2} \supset A_{n-1} \supset A_{n} \subset A$ in which case $A \cup A_i = A \cup A_{i+1}$ and $A \cup A_{n} = A$; (iv) $A_1 \supset A_2 \supset \ldots \supset A_{n-2} \supset A_{n-1} \supset A_{n} \subset A$. Hence, for the first three cases at most $n-2$ new subsets of the form $A_i \cup A$ out of all subset of $A_i \cup A , 1 \leq i \leq n$ plus one new subset $A$ are generated. Otherwise, in case (iv) the possible different subsets are only in the form of $A_1, A_2, \ldots, A_n, A \cup A_1, A \cup A_2, \ldots, A \cup A_n$ which are 2n in total.

\emph{Claim 3:} Let $F_n$ is the maximum number of elements in the $|(\mathcal{A})^2|$ where $|A| = n$. It can be directly checked for the small number of $n \leq 5$ that $F_1 = F_2 = F_3 = 1$, $F_4 = 5$, and $F_5 = 8$. Based on the results of claim 1 and 2, we can prove that $F_{n+2} \leq F_n + 2n - 2$, hence we have
\begin{align}
    \left\{ \begin{array}{ll}
        F_n \leq \frac{n(n-4)}{2}+5, & n = 2b, n \geq 4 \\
        F_n \leq \frac{(n+1)(n-5)}{2}+8, & n = 2b-1, n \geq 5 
    \end{array}
    \right.
\end{align}

\emph{Claim 4:} Let $\mathcal{A}_i = \{A \in \mathcal{C}, i \in A\}$ and $n_i = |\mathcal{A}_i|$. Obviously the set of component beams in $\mathcal{A}_i= \{A_1, A_2, \ldots, A_{n_i}\}$ are sequentially in order on the loop. Let $n$ be the maximum value of $n_i$ and correspondingly $\mathcal{A} = \mathcal{A}_i$ and $\mathcal{D} = \mathcal{C} - \mathcal{A}_i$. Assume the elements of $\mathcal{A} = \{A_1, \ldots, A_n\}$ and $\mathcal{D} = \{D_1, \ldots, D_m\}$ are in order on the loop such that $D_1$ and $D_m$ are the neighbors of $A_n$, $A_1$, respectively. We have $n+m=2b$.
Since $D_m \subset A_1$ and for the $i$ which maximizes $n_i$ we have $i \in A_1$ but $i \notin D_m$, hence $D_m \subset A_1$. Similarly we have and $D_1 \subset A_{n_i}$, which means that for all $k = 1, 2, \ldots, n_i$, we have $D_m A_i = A_1 A_i$ and $D_1 A_i = A_{n_i} A_i$. This means that there are $2n_i$ elements in $\mathcal{A} \times \mathcal{D}$ which is in common with elements in $\mathcal{A}^2$.

If there is $n_i \geq 6$ then we have $|\mathcal{A} \times \mathcal{D}| \leq n_i  (2b-n_i) - 2  n_i$ and for even $n_i$ we have
\begin{align}
    |\mathcal{C}^2| &\leq |\mathcal{A}^2| + |\mathcal{D}^2| + |\mathcal{A} \times \mathcal{D}|\\
    &\leq (\frac{(n_i)(n_i - 4)}{2}+5) + (\frac{(2b-n_i)(2b-n_i - 4)}{2}+5) \nonumber \\
    &+ (n_i  (2b-n_i) - 2  n_i) < 2b(b-2),
\end{align}
and for odd $n_i$ we have
\begin{align}
    |\mathcal{C}^2| & \leq (\frac{(n_i+1)(n_i - 5)}{2}+8) + \nonumber \\ 
    &(\frac{(2b-n_i+1)(2b-n_i - 5)}{2}+8)  \nonumber \\ 
    &+ (n_i  (2b-n_i) - 2  n_i) < 2b(b-2). 
\end{align}
Hence, the maximal design cannot have $n_i \geq 6$ since for Tulip structure $|\mathcal{C}^2| = 2b(b-2)$.

\emph{Claim 5:} Next, assume that $n_i = 5$. We note that $D_1$ cannot be a subset $D_m$, otherwise there is a beam which is in at least $6$ consecutive component beams $A_n, D_1, D_2, \ldots, D_m$. Hence, we can find a minimum index $1 < k \leq m$ such that $D_1 \not \subset D_k$ for which we have $A_n D_k = A_n D_{k-1}$. Similarly, we have a minimum index $l$ such that $D_m \not \subset D_l$ for which we have $A_1 D_l = A_1 D_{l-1}$. 
On the other hand, there is a maximum index $1 \leq j < n$ such that $D_1 \not \subset A_j$ otherwise there is a common beam in at least 6 consecutive component beams $A_1, A_2, \ldots, A_n, D_1$. Hence we have $D_1 A_j = D_1 A_{j-1}$. Similarly there a minimal index $t$ such that $D_m \not \subset A_t$ otherwise there is a common beam in at least $6$ consecutive component beams $D_m, A_1, A_2, \ldots, A_n$. Hence we have $D_m A_t = D_m A_{t-1}$.
This means we have $|\mathcal{A} \times \mathcal{D}| \leq 5  (2b-5) - 2 \times 5 - 4$ and
\begin{align}
    |\mathcal{C}^2| & \leq (8) + (\frac{(2b-4)(2b- 10)}{2}+8)  \nonumber \\ 
    &+ (5  (2b-5) - 14) < 2b(b-2). 
\end{align}
Hence, the maximal design cannot have $n_i \geq 5$ since for Tulip structure $|\mathcal{C}^2| = 2b(b-2)$.

\emph{Claim 6:} Next, assume that $n_i = 4$. This case is very similar to the Claim 5 for $n_i = 5$ which the exception that we use the formula of $F_n$ for the even $n$. We note that $D_1$ cannot be a subset $D_m$, otherwise there is a beam which is in at least $5$ consecutive component beams $A_n, D_1, D_2, \ldots, D_m$. Hence, we can find a minimum index $1 < k \leq m$ such that $D_1 \not \subset D_k$ for which we have $A_n D_k = A_n D_{k-1}$. Similarly, we have a minimum index $l$ such that $D_m \not \subset D_l$ for which we have $A_1 D_l = A_1 D_{l-1}$. 
On the other hand, there is a maximum index $1 \leq j < n$ such that $D_1 \not \subset A_j$ otherwise there is a common beam in the at least $5$ consecutive component beams $A_1, A_2, \ldots, A_n, D_1$. Hence we have $D_1 A_j = D_1 A_{j-1}$. Similarly there a minimal index $t$ such that $D_m \not \subset A_t$ otherwise there is a common beam in at least $5$ consecutive component beams $D_m, A_1, A_2, \ldots, A_n$. Hence we have $D_m A_t = D_m A_{t-1}$.
This means we have $|\mathcal{A} \times \mathcal{D}| \leq 4  (2b-4) - 2 \times 4 - 4$ and
\begin{align}
    |\mathcal{C}^2| & \leq (5) + (\frac{(2b-4)(2b-8)}{2}+5)  \nonumber \\ 
    &+ (4  (2b-4) - 12) < 2b(b-2). 
\end{align}
Hence, the maximal design cannot have $n_i \geq 4$ since for Tulip structure $|\mathcal{C}^2| = 2b(b-2)$.

On the one hand, the max $n_i$ is less than or equal to 3. On the other hand for all $C_i$ in $\mathcal{C}$, $|C_i| \geq 1$ and for every two consecutive $C_i$ and $C_{i+1}$ we have $|C_i| = |C_{i+1}| \geq 3$. Hence, 
$$\sum_{i=1}^{b} n_i = \sum_{i=1}^{2b} |C_i| >= 3b$$
which means that all $n_i$ have to be equal to 3. This means that Tulip structure is maximal and indeed the unique optimal solution.

%\begin{thm}
%A set of scanning beams with flower design (defined earlier?) generates the maximal number of possible feedback sequences. For $p > 1$, %flower design is the only?? maximal set?
%\label{thm: flower}
%\end{thm}
